# Supplementary material for: Fast variational Bayes methods for multinomial probit models
Source: arXiv:2202.12495 source file (2022-10-15)
Supplement: Supplementary file 1 [file web_appendix.tex]

\appendix
\newpage
\noindent
\setcounter{page}{1}
\begin{center}
	{\bf \Large{Online Appendix for ` Title of the paper'}}
\end{center}

\vspace{10pt}

\setcounter{figure}{0}
\setcounter{table}{0}
\setcounter{section}{0}

\noindent
This Online Appendix has xxxx parts:
\begin{itemize}
    \item[] {\bf Part~A}: Derivation of expressions required for variational inference.
	\item[] {\bf Part~B}:  .

\end{itemize}
\newpage
\section{Computing gradients}\label{App:VIdetails}

After transforming all the parameters to the real line, we have that $\bm{\theta} = \left(\bm{\beta}^\top,\bm{\xi}^\top\right)^\top$, where $\bm{\xi} = \left(\bm{\xi}_1^\top,\dots,\bm{\xi}_K^\top\right)^\top$ and $\bm{\xi}_k = \left(\xi_{k,1},\dots,\xi_{k,n_k-1}\right)^\top$. 
With this new notation, the function $\log g(\bm{\theta},\bm{z})$ can be written as 
\begin{equation}
 \log g(\bm{\theta},\bm{z}) = \log p(\bm{y}|\bm{z})+ \log p(\bm{\theta})+\sum_{i=1}^{N}\log \phi_{J}\left(\bm{z}_i;X_i\bm{\beta},\Sigma(\bm{\xi})\right),
\end{equation}
where 
\begin{equation}
 \log p(\bm{\theta}) = \log p(\bm{\beta})+\sum_{k=1}^{K}\sum_{l=1}^{n_k-1}\log p(\xi_{k,l}),
\end{equation}
and $\Sigma(\bm{\xi})$ reflects the fact that the covariance matrix now depends on $\bm{\xi}$.
To conduct variational inference we must construct the gradient $\nabla_{\theta}\log g(\bm{\theta},\bm{z}) = \left(\nabla_{\beta}\log g(\bm{\theta},\bm{z})^\top,\nabla_{\xi}\log g(\bm{\theta},\bm{z})^\top\right)^\top$, where 
\begin{equation}\label{Eq:grad1}
    \nabla_{\beta}\log g(\bm{\theta},\bm{z}) = \nabla_{\beta}\log p(\bm{\theta})+\sum_{i=1}^{N}\nabla_{\beta}\log \phi_{J}\left(\bm{z}_i;X_i\bm{\beta},\Sigma(\bm{\xi})\right)
\end{equation}
and
\begin{equation}\label{Eq:grad2}
    \nabla_{\xi}\log g(\bm{\theta},\bm{z}) = \nabla_{\xi}\log p(\bm{\theta})+\sum_{i=1}^{N}\nabla_{\xi}\log \phi_{J}\left(\bm{z}_i;X_i\bm{\beta},\Sigma(\bm{\xi})\right)
\end{equation}
Below we derive the four expression required to evaluate the gradients in \eqref{Eq:grad1} and \eqref{Eq:grad2}. Throughout we use $\bm{\eta}_i = \bm{z}_i-X_i\bm{\beta}$.

\subsection{Computing $\nabla_{\beta}\log p(\bm{\theta})$}
$$\nabla_{\beta}\log p(\bm{\theta}) = -\frac{1}{10}\bm{\beta}$$
\subsection{Computing $\nabla_{\xi}\log p(\bm{\theta})$}
To compute this gradient we know that
$\nabla_{\xi}\log p(\bm{\theta}) = \left(\nabla_{\xi_1}\log p(\bm{\theta})^\top,\dots,\nabla_{\xi_K}\log p(\bm{\theta})^\top\right)^\top$, where 
$$\nabla_{\xi_k}\log p(\bm{\theta}) = \left(\frac{\partial \log p(\xi_{k,1})}{\partial \xi_{k,1}},\dots,\frac{\partial \log p(\xi_{k,n_k-1})}{\partial \xi_{k,n_k-1}}\right)^\top,$$
and 
$$\frac{\partial \log p(\xi_{k,l})}{\partial \xi_{k,l}} = -\frac{1}{\hat{\tau}_{k,l}}t_{\hat{\eta}_{k,l}}\left[\frac{\xi_{k,l}-\hat{\mu}_{k,l}}{\hat{\tau}_{k,l}}\right]t_{\hat{\eta}_{k,l}}'\left[\frac{\xi_{k,l}-\hat{\mu}_{k,l}}{\hat{\tau}_{k,l}}\right]+\frac{1}{\hat{\tau}_{k,l}}\frac{t_{\hat{\eta}_{k,l}}''\left[\frac{\xi_{k,l}-\hat{\mu}_{k,l}}{\hat{\tau}_{k,l}}\right]}{t_{\hat{\eta}_{k,l}}'\left[\frac{\xi_{k,l}-\hat{\mu}_{k,l}}{\hat{\tau}_{k,l}}\right]}.$$
Closed-form expressions for $t_{\hat{\eta}_{k,l}}(\cdot)$, $t_{\hat{\eta}_{k,l}}'(\cdot)$ and $t_{\hat{\eta}_{k,l}}''(\cdot)$ are provided in Table 1 in \cite{smith2020high}.

\subsection{Computing $\nabla_{\beta}\log \phi_{J}\left(\bm{z}_i;X_i\bm{\beta},\Sigma(\bm{\xi})\right)$}
\begin{align}
    \nabla_{\beta}\log \phi_{J}\left(\bm{z}_i;X_i\bm{\beta},\Sigma(\bm{\xi})\right)^\top& = \bm{\eta}_i^\top\Sigma^{-1}X_i
\end{align}
\subsection{Computing $\nabla_{\xi}\log \phi_{J}\left(\bm{z}_i;X_i\bm{\beta},\Sigma(\bm{\xi})\right)$}
To compute this last term we must use the chain rule of derivatives. To deal with these operations, we will use the convention that for two generic matrices $C_{\text{dim1}\times\text{dim2}}$ and $L_{\text{dim3}\times\text{dim4}}$ we have that
$$\frac{\partial C}{\partial L} = \frac{\partial \text{vec}(C)}{\partial \text{vec}(L)} = E$$
where $E$ is of dimension $(\text{dim1}*\text{dim2})\times(\text{dim3}*\text{dim4})$.
With this definition, we can then write the gradient of interest as
\begin{align}
    \nabla_{\xi}\log \phi_{J}\left(\bm{z}_i;X_i\bm{\beta},\Sigma(\bm{\xi})\right)^\top &= \frac{\partial}{\partial \bm{\xi}}\left[-\frac{J}{2}\log(2\pi)-\frac{1}{2}\log (\text{det}(\Sigma))-\frac{1}{2}\bm{\eta}_i^\top\Sigma^{-1}\bm{\eta}_i\right]\nonumber\\
    & =  -\frac{1}{2}\frac{\partial}{\partial \bm{\xi}}\log (\text{det}(\Sigma))-\frac{1}{2}\frac{\partial}{\partial \bm{\xi}}\bm{\eta}_i^\top\Sigma^{-1}\bm{\eta}_i\nonumber\\
    & =  -\frac{1}{2}\frac{1}{\text{det}(\Sigma)}\frac{\partial \text{det}(\Sigma)}{\partial \Sigma}\frac{\partial \Sigma}{\partial \bm{\xi}}-\frac{1}{2}\frac{\partial}{\partial \bm{\xi}}\bm{\eta}_i^\top\Sigma^{-1}\bm{\eta}_i\nonumber \\
    & =  -\frac{1}{2}\frac{1}{\text{det}(\Sigma)}\frac{\partial \text{det}(\Sigma)}{\partial \Sigma}\frac{\partial \Sigma}{\partial \bm{\xi}}-\frac{1}{2}\left(\bm{\eta}_i^\top\otimes\bm{\eta}_i^\top\right)\frac{\partial}{\partial \bm{\xi}}\text{vec}(\Sigma^{-1})\nonumber\\
     & =  -\frac{1}{2}\frac{1}{\text{det}(\Sigma)}\frac{\partial \text{det}(\Sigma)}{\partial \Sigma}\frac{\partial \Sigma}{\partial \bm{\xi}}-\frac{1}{2}\left(\bm{\eta}_i^\top\otimes\bm{\eta}_i^\top\right)\frac{\partial \Sigma^{-1}}{\partial \Sigma}\frac{\partial \Sigma}{\partial \bm{\xi}}\nonumber\\
     & =  -\frac{1}{2}\frac{1}{\text{det}(\Sigma)}\frac{\partial \text{det}(\Sigma)}{\partial \Sigma}\frac{\partial \Sigma}{\partial B}\frac{\partial B}{\partial\bm{\kappa}}\frac{\partial \bm{\kappa}}{\partial \bm{\xi}}-\frac{1}{2}\frac{1}{\text{det}(\Sigma)}\frac{\partial \text{det}(\Sigma)}{\partial \Sigma}\frac{\partial \Sigma}{\partial \bm{d}}\frac{\partial \bm{d}}{\partial\bm{\kappa}}\frac{\partial \bm{\kappa}}{\partial \bm{\xi}}\nonumber\\
     &\hspace{0.7cm}-\frac{1}{2}\left(\bm{\eta}_i^\top\otimes\bm{\eta}_i^\top\right)\frac{\partial \Sigma^{-1}}{\partial \Sigma}\frac{\partial \Sigma}{\partial B}\frac{\partial B}{\partial\bm{\kappa}}\frac{\partial \bm{\kappa}}{\partial \bm{\xi}}-\frac{1}{2}\left(\bm{\eta}_i^\top\otimes\bm{\eta}_i^\top\right)\frac{\partial \Sigma^{-1}}{\partial \Sigma}\frac{\partial \Sigma}{\partial \bm{d}}\frac{\partial \bm{d}}{\partial\bm{\kappa}}\frac{\partial \bm{\kappa}}{\partial \bm{\xi}}\nonumber
\end{align}
where we used the fact that $\frac{\partial \Sigma}{\partial \bm{\xi}} = \frac{\partial \Sigma}{\partial B}\frac{\partial B}{\partial \bm{\kappa}}\frac{\partial \bm{\kappa}}{\partial \bm{\xi}}+\frac{\partial \Sigma}{\partial \bm{d}}\frac{\partial \bm{d}}{\partial \bm{\kappa}}\frac{\partial \bm{\kappa}}{\partial \bm{\xi}}$. All we have to do to now is to find an expression for each of the derivatives required for $\nabla_{\xi}\log \phi_{J}\left(\bm{z}_i;X_i\bm{\beta},\Sigma(\bm{\xi})\right)$. We derive each of these expressions below.

\ \\
\textbf{Derivation of } $\frac{1}{2}\left(\bm{\eta}_i^\top\otimes\bm{\eta}_i^\top\right)\frac{\partial \Sigma^{-1}}{\partial \Sigma}\frac{\partial \Sigma}{\partial B}$\\
\ \\
Denote as $K_{J,J}$ the commutation matrix so that $K_{J,J}\text{vec}(\Sigma)=\text{vec}(\Sigma^\top)$. The two derivative terms can be written as
$$\frac{\partial \Sigma^{-1}}{\partial \Sigma} = -\left(\Sigma^{-\top}\otimes\Sigma^{-1}\right)$$
$$\frac{\partial \Sigma}{\partial B} = \left(I_{J^2}+K_{J,J}\right)\left(B\otimes I_J\right).$$
The product of these two derivatives can be simplified as
$$\frac{\partial \Sigma^{-1}}{\partial \Sigma}\frac{\partial \Sigma}{\partial B} = -\left(I_{J^2}+K_{J,J}\right)\left(\Sigma^{-1}B\otimes\Sigma^{-1}\right)$$
Finally 
\begin{align}
    \frac{1}{2}\left(\bm{\eta}_i^\top\otimes\bm{\eta}_i^\top\right)\frac{\partial \Sigma^{-1}}{\partial \Sigma}\frac{\partial \Sigma}{\partial B}&=-\frac{1}{2}\left(\bm{\eta}_i^\top\otimes\bm{\eta}_i^\top\right)\left(I_{J^2}+K_{J,J}\right)\left(\Sigma^{-1}B\otimes\Sigma^{-1}\right)\\
    & =-\frac{1}{2}\left(\bm{\eta}_i^\top\Sigma^{-1}B\otimes\bm{\eta}_i^\top\Sigma^{-1}\right)-\frac{1}{2}\left(\bm{\eta}_i^\top\Sigma^{-1}\otimes\bm{\eta}_i^\top\Sigma^{-1}B\right)K_{J,q}\\
    & = -\left(\bm{\eta}_i^\top\Sigma^{-1}B\otimes\bm{\eta}_i^\top\Sigma^{-1}\right)
\end{align}
\ \\
\textbf{Derivation of } $\frac{1}{2}\left(\bm{\eta}_i^\top\otimes\bm{\eta}_i^\top\right)\frac{\partial \Sigma^{-1}}{\partial \Sigma}\frac{\partial \Sigma}{\partial \bm{d}}$\\
Following identical steps as above we can show that 
\begin{align}
    \frac{1}{2}\left(\bm{\eta}_i^\top\otimes\bm{\eta}_i^\top\right)\frac{\partial \Sigma^{-1}}{\partial \bm{d}}
    & = -\left(\bm{\eta}_i^\top\Sigma^{-1}D\otimes\bm{\eta}_i^\top\Sigma^{-1}\right)P,
\end{align}
where $P$ extracts the columns correspoding to the elements of $\bm{d}$.\\
\ \\
\textbf{Derivation of } $\frac{\partial B}{\partial \bm{\kappa}}$\\
Let us define as $A = \left[A_1^\top |\dots| A_K^\top\right]^\top$. Note that $B = AP_1$, $\bm{d} = AP_2$ for $P_1 = [\bm{0}_{q\times 1}|I_{q}]^T$ and $P_2 = \left(1,\bm{0}_{1\times q}\right)^\top$. With this notation we can then write
$$\frac{\partial B}{\partial \bm{\kappa}}=\frac{\partial B}{\partial A^\top}\frac{\partial A^\top}{\partial \bm{\kappa}}.$$
The first term can be derived from the expression
\begin{align}
    \text{vec}\left(B\right)&=\left(P_1^\top\otimes I_{J}\right)\text{vec}\left(A\right)=\left(P_1^\top\otimes I_{J}\right)K_{q+1,J}\text{vec}\left(A^\top\right)
\end{align}
from which we obtain 
$$\frac{\partial B}{\partial A^\top}=\left(P_1^\top\otimes I_J\right)K_{q+1,J}.$$
The second term is the block matrix
$$\frac{\partial A^\top}{\partial \bm{\kappa}} = \text{blockdiag}\left(\frac{\partial A_1^\top}{\partial \bm{\kappa}_1},\dots,\frac{\partial A_K^\top}{\partial \bm{\kappa}_K}\right),$$
where, denoting the element in the $j$th row and $l$th column of $\frac{\partial A_k^\top}{\partial \bm{\kappa}_k}$ as 
$\left\{\frac{\partial A_k^\top}{\partial \bm{\kappa}_k}\right\}_{j,l}$, then 

{\footnotesize
\[
\left\{\frac{\partial A_k^\top}{\partial \bm{\kappa}_k}\right\}_{j,l} =
\left\{\begin{array}{cl}
\sqrt{J_k}\cos\left(\kappa_{k,j}\right)\cos\left(\kappa_{k,l}\right)\prod_{s\in\{1,\dots,j-1\}\backslash l}\sin\left(\kappa_{k,s}\right) &\text{If} \ \ \ \ l<j\ \ \wedge\ \  j<n_k\\
-\sqrt{J_k}\prod_{s=1}^{l}\sin\left(\kappa_{k,s}\right) &\text{If} \ \ \ \ l=j\ \ \wedge\ \  j<n_k\\
\sqrt{J_k}\cos\left(\kappa_{k,l}\right)\prod_{s\in\{1,\dots,k\}\backslash l}\sin\left(\kappa_{k,s}\right) &\text{If} \ \ \ \ l<n_k-1\ \ \wedge\ \  j=n_k\\
\sqrt{J_k}\cos\left(\kappa_{k,l}\right)\prod_{s=1}^{l-1}\sin\left(\kappa_{k,s}\right) &\text{If} \ \ \ \ l=n_k-1\ \ \wedge\ \  j=n_k\\
0 &\text{Otherwise}\\
\end{array} \right.
\]
}
\ \\
\textbf{Derivation of }$\frac{\partial \bm{d}}{\partial \bm{\kappa}}$\\
Similarily, we have that
$$\frac{\partial \bm{d}}{\partial \bm{\kappa}}=\frac{\partial \bm{d}}{\partial A^\top}\frac{\partial A^\top}{\partial \bm{\kappa}}$$
We calculated the second term previously. Following the same logic as before, the first term can be computed from noting that
$$\text{vec}\left(\bm{d}\right)=\left(P_2^\top\otimes I_J\right)\text{vec}\left(A\right)=\left(P_2^\top\otimes I_J\right)K_{q+1,J}\text{vec}\left(A^\top\right)$$
so that 
$$\frac{\partial \bm{d}}{\partial A^\top}=\left(P_2^\top\otimes I_J\right)K_{q+1,J}$$

\ \\
\textbf{Other terms required}\\

$$\frac{\partial \text{det}(\Sigma)}{\partial \Sigma} = \text{det}(\Sigma)\text{vec}(\Sigma^{-1})^\top$$
